# Supplementary material for: Particle-In-Cell Simulations of Quantum Plasmas
Source: arXiv:2501.07465 ancillary file (2025-01-13)
Supplement: Supplementary file 1 [file Quantum_Plasma_Supplemental_Information.pdf]

# Particle-In-Cell Simulations of Quantum Plasmas, Supplemental Information

Gregory K. Ngirmang[a,1,*], Hue T.B. Do[b,1], Guangxin Liu[a], Michel Bosman[b], Lin Wu[a,*]

[a]*Science, Mathematics, and Technology Pillar, Singapore University of Technology and Design, 8 Somapah Road, Singapore 487372*
[b]*Department of Materials Science and Engineering, National University of Singapore, 9 Engineering Drive 1, Singapore 117575*

## S1. PIC Simulation Parameters

Table S1 summarizes the simulation parameters for the PIC studies presented in the main text. All simulations employ second-order explicit schemes for fields, interpolation, and current deposition, as specified by the respective codes. The simulations use cubic (or square) cells, and only the spatial cell size along the $x$-axis, $\Delta x$, is reported. Key details for specific simulations are as follows:

- Section 3, Figs. 3C, 3D: An electron beam with a weight of 3.5 $\mathrm{nm}^{-1}$, moving at $0.5c$ along the $x$-axis, is used to stimulate the structure for studying its frequency response.
- Section 4, Fig. 6: A tightly focused Gaussian pulse is injected along the $x$-axis, and the reflectivity is analyzed to obtain the spectral response shown in this figure. Figs. 7 and S3: An electron beam with a density of $10^{26}$ $\mathrm{m}^{-3}$ is injected along the $x$-axis to generate emission from the target. For these simulations, both bound particle species are initialized with one particle per cell at the center. In Fig. 6, there are 4 particles per cell (1 per species), while in Fig. 7, there is 1 particle per cell.
- Section 5, Fig. 8: A beam consisting of 1000 particles, each with the charge of an electron, drifts in the $z$-direction with velocity $v_z = 0.5c$, exciting the graphene structures.

*Corresponding authors
*Email addresses:* ngirmang@protonmail.com (Gregory K. Ngirmang), lin_wu@sutd.edu.sg (Lin Wu)
[1]Gregory K. Ngirmang and Hue T. B. Do are equally the first authors of this work

| section | code | dimensionality | $\Delta x$ | $\Delta t$ | boundary conditions | particles per cell |
|---|---|---|---|---|---|---|
| Sec. 2, Fig. 2 | EPOCH | 3D | 0.2 nm | 0.95 $\Delta t_{\rm CFL}$ | all periodic | from 8 to 1024 |
| Sec. 3, Fig. 3A,3B | Smilei | 2D | 0.05 nm | 0.5 $\Delta t_{\rm CFL}$ | $x$:absorbing, $y$:periodic | 64 |
| Sec. 3, Fig. 3C,3D | Smilei | 2D | 0.1 nm | 0.5 $\Delta t_{\rm CFL}$ | $x$:absorbing, $y$:periodic | 64 |
| Sec. 4, Fig. 6 | EPOCH | 3D | 1 nm | 0.95 $\Delta t_{\rm CFL}$ | $x$:absorbing, $y$,$z$:periodic | 1 per species (4 species) |
| Sec. 4, Fig. 7 | EPOCH | 2D | 5 nm | 0.95 $\Delta t_{\rm CFL}$ | all absorbing | 1 |
| Sec. 5, Fig. 8 | Smilei | 3D | 1 nm | 0.9 $\Delta t_{\rm CFL}$ | $x$,$y$:periodic; $z$:absorbing | 10×10 in $x$ and $y$, 1 in $z$ |

Table S1: PIC parameters used for in the simulation studies presented in this work. In this table, $\Delta t$ is the timestep, $\Delta t_{\rm CFL}$ is the CFL [1] limited time step, and $\Delta x$ is the grid spacing along the $x$ axis.

## S2. Electron dynamics near metallic edges

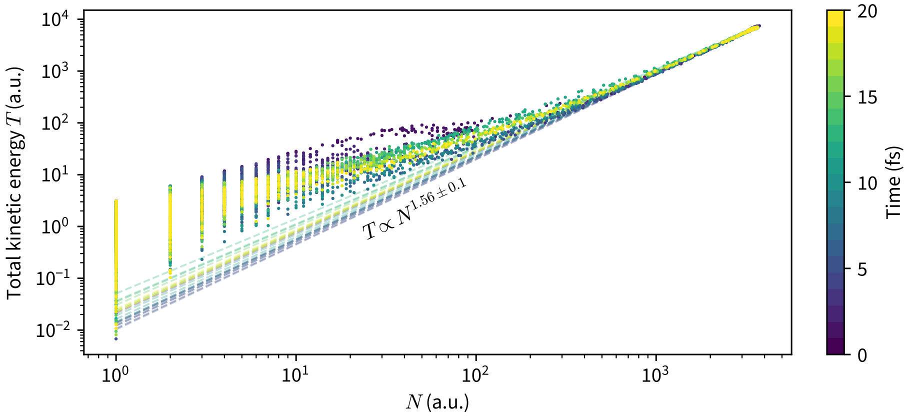


Figure S1: Total kinetic energy $T$ versus electron density $N$ across the material boundary of Na, corresponding to $r_s = 4$ (green data in Figure 3a) during electron spill-out transient time. The dashed lines show the fitting of $T \propto N^x$

## S3. Lorentzian fit for silicon dielectric function

The parameters used to fit the silicon dielectric function found in Dong et al. [2], displayed in Fig. S2 are summarised in Table S2, and this model for silicon is used for Fig. 6 in the main text. The parameters are defined in the main text, Eq. (7). Here, the dielectric function is taken to be isotropic, so the tensorial nature of $\varepsilon(\omega)$ can be ignored.

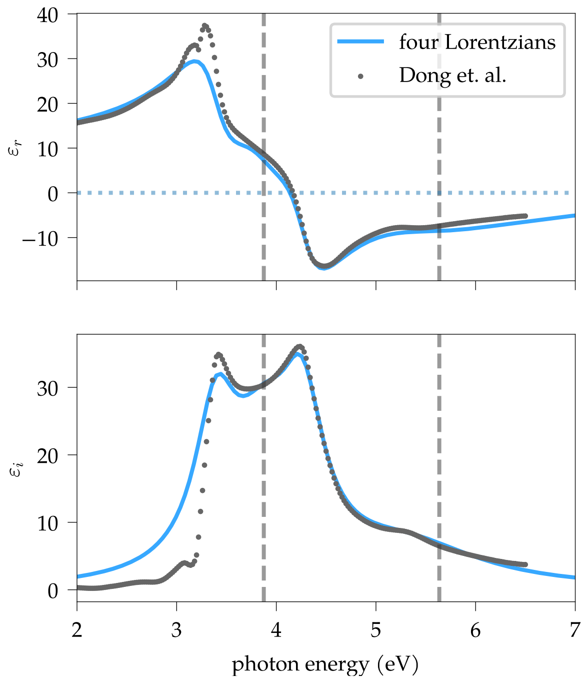


Figure S2: Fitting of four Lorentzians to the dielectric function of silicon from [2].

| label | density ($m^{-3}$) | $\hbar\omega_p$ | $\hbar\omega_b$ | $\hbar\gamma_b$ |
|---|---|---|---|---|
| $E_0$ | $4.41 \cdot 10^{28}$ | 7.8 | 3.9 | 0.84 |
| $E_1$ | $2.61 \cdot 10^{28}$ | 6.0 | 3.4 | 0.5 |
| $E_2$ | $3.16 \cdot 10^{28}$ | 6.6 | 4.27 | 0.5 |
| $E_1'$ | $3.97 \cdot 10^{28}$ | 7.4 | 5.4 | 1.8 |

Table S2: The four resonances used to fit the dielectric function of silicon from [2]. All parameters except for density are specified in electron volts.

## S4. Emission from electron bunch transition through a constant dielectric

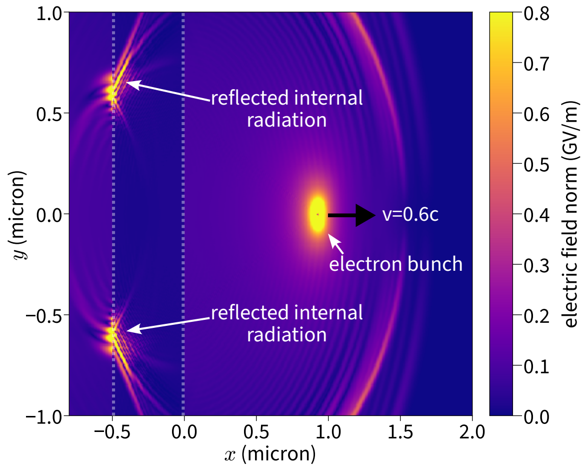


Figure S3: Transition of an electron bunch moving at $0.6c$ through a constant dielectric barrier with radiation emission, to be compared to Fig. 7 in the main text. The bulk bound waves are absent, although internal radiation that originated from the exit of the charge is visible, whereas in Fig. 7 these waves have dissipated.

## References


[1] R. Courant, K. Friedrichs, H. Lewy, Über die partiellen differenzengleichungen der mathematischen physik, Mathematische Annalen 100 (1928) 32–74. doi:10.1007/BF01448839.

[2] Z. Dong, T. Wang, X. Chi, J. Ho, C. Tserkezis, S. L. K. Yap, A. Rusydi, F. Tjiptoharsono, D. Thian, N. A. Mortensen, J. K. W. Yang, Ultraviolet interband plasmonics with si nanostructures, Nano Letters 19 (11) (2019) 8040–8048. doi:10.1021/acs.nanolett.9b03243.
